# Supplementary material for: SimBa: Simplicity Bias for Scaling Up Parameters in Deep Reinforcement Learning
Source: arXiv:2410.09754 source file (2025-05-29)
Supplement: Supplementary file 1 [file appendix_simba_different_architecture.pdf]

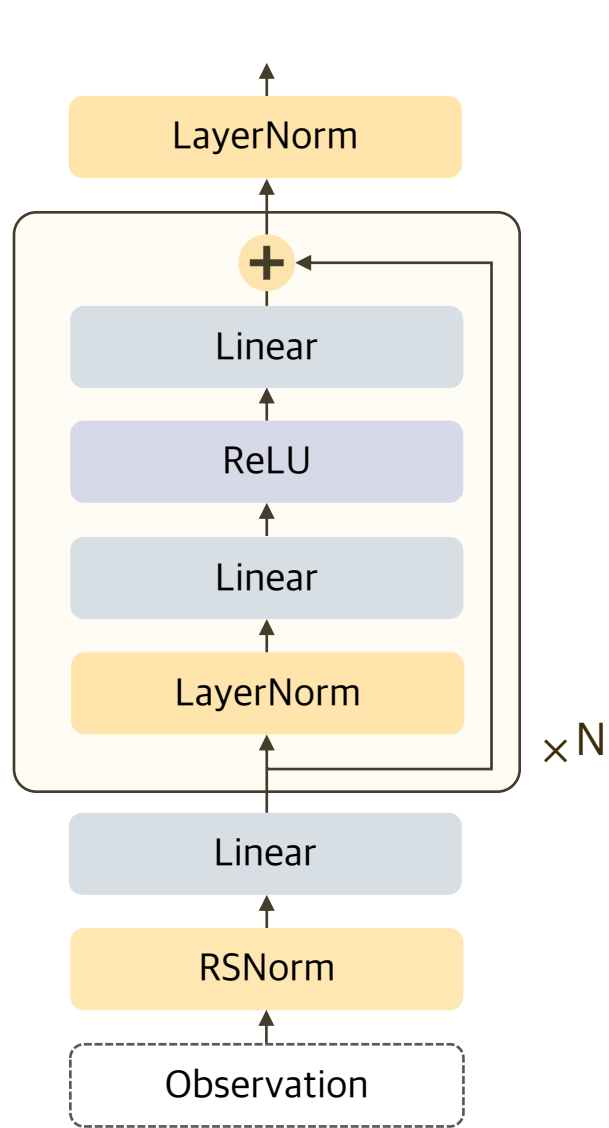

(a) SimBa

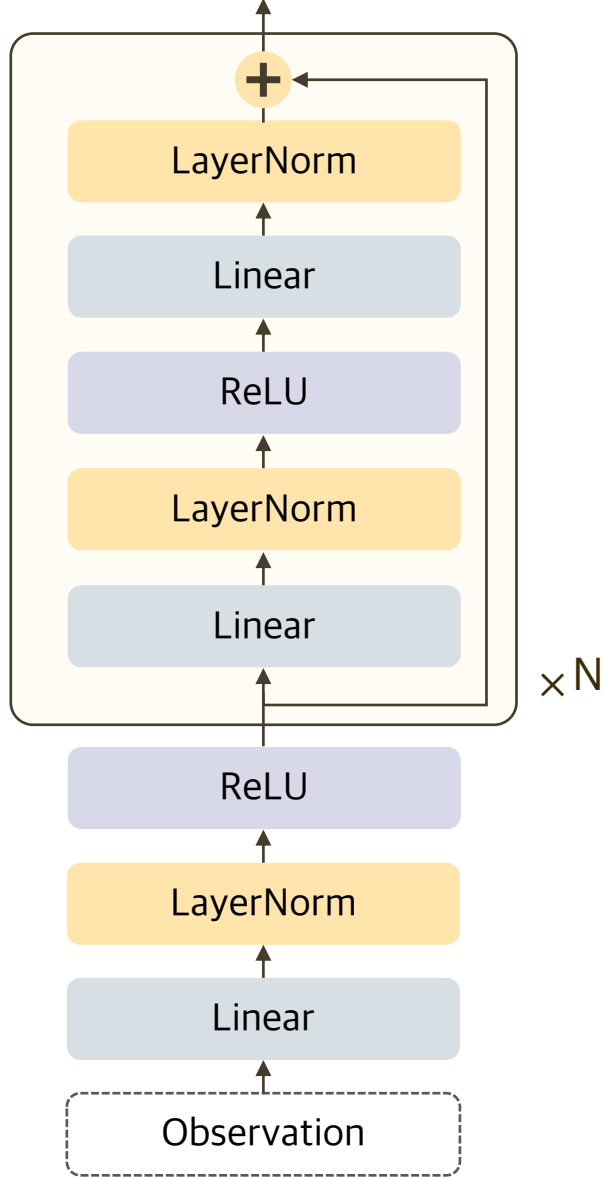

(b) BroNet

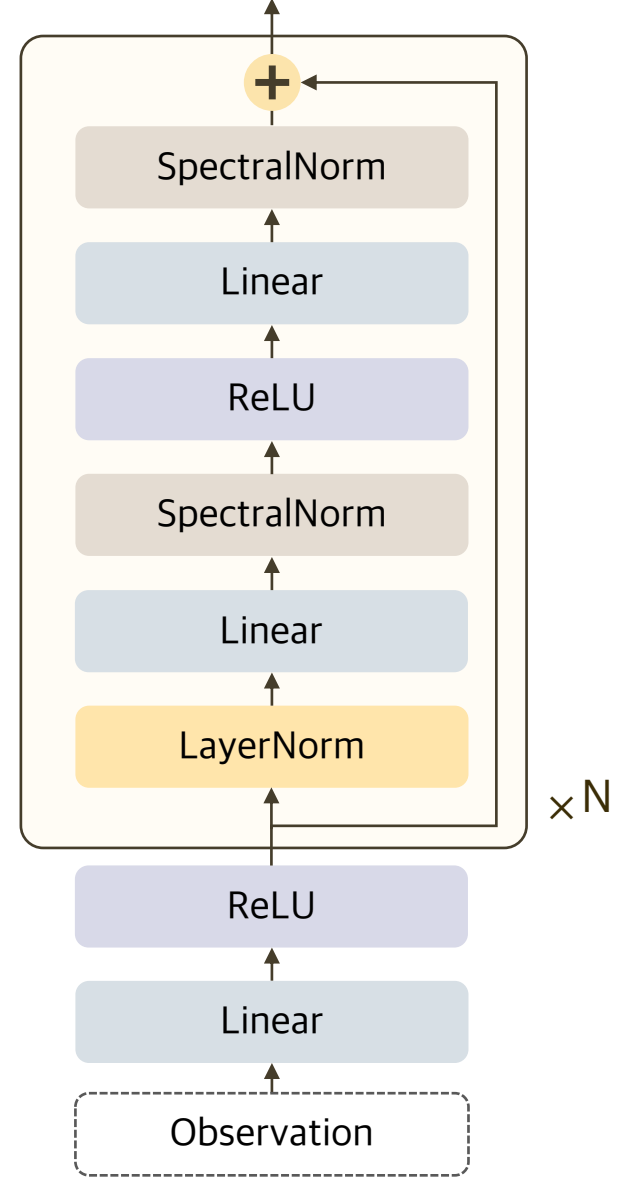

(c) SpectralNet

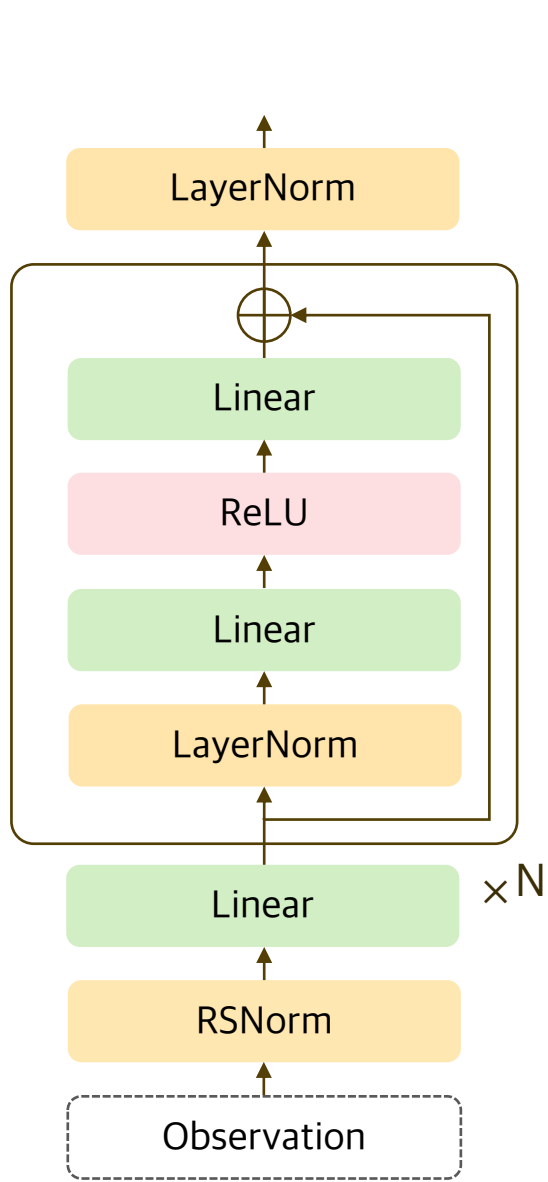

(a) SimBa

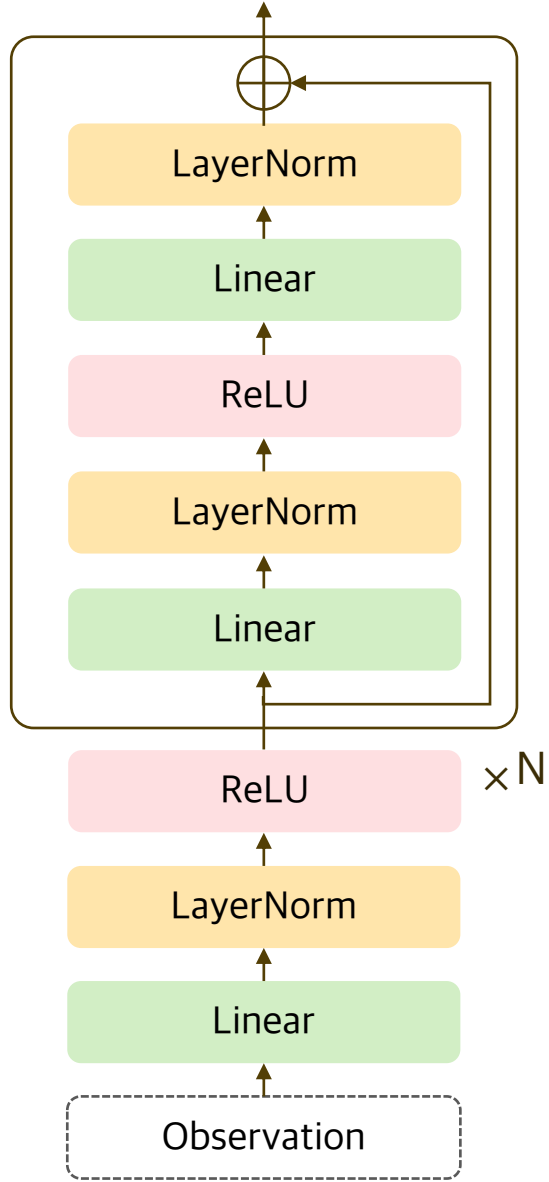

(b) BroNet

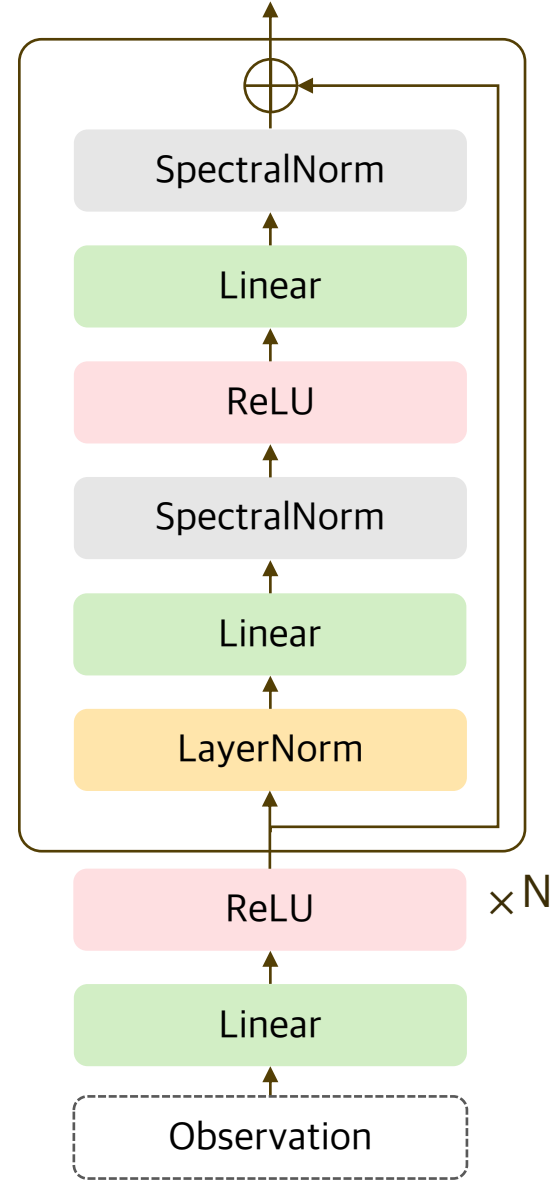

(c) SpectralNet
